# Supplementary material for: Inference for two-stage sampling designs with application to a panel for urban policy
Source: arXiv:1808.09758 source file (2019-01-04)
Supplement: Supplementary file 1 [file SupplementaryMaterial_v8_HAL.pdf]

# Consistency of estimators and variance estimators for two-stage sampling

## Supplementary Material

Guillaume Chauvet[(1)] and Audrey-Anne Vallée[(2)]
[(1)] Ensai (Irmar), Campus de Ker Lann, Bruz - France
[(2)] Institut de Statistique, Université de Neuchâtel, Switzerland

December 14, 2018

## 1 Some moments inequalities

The proof of the following Lemmas is standard, and is therefore omitted.

**Lemma 1.** *Suppose that Assumptions (FS1) and (FS2) hold. There exists some constant $C'_{I5}$ such that*

$$\max_{i\neq j\neq i'\neq j'=1,\ldots,N_I} |\Delta_{Iij,i'j'}| \;\leq\; C'_{I5} N_I^{-4} n_I^3, \tag{A1}$$

*with $\Delta_{Iij,i'j'} = Cov(I_{Ii}I_{Ij}, I_{Ii'}I_{Ij'})$.*

**Lemma 2.** *Suppose that Assumptions (SS1) and (SS2) hold. There exists some constant $C'_5$ such that*

$$\max_{i\in U_I} \max_{k\neq l\neq k'\neq l'=1,\ldots,N_i} \left|\Delta_{kl,k'l'|i}\right| \;\leq\; C'_5 N_0^{-4} n_0^3, \tag{A2}$$

*with $\Delta_{kl,k'l'|i} = Cov(I_kI_l, I_{k'}I_{l'}|i \in S_I)$.*

**Lemma 3.** *Under Assumptions (SS0) and (VAR1), there exists some constant $M$ such that*

$$N_I^{-1}\sum_{i=1}^{N_I} Y_i^4 \;\leq\; M\; N_0^4. \tag{A3}$$

**Lemma 4.** *Under Assumptions (SS0)-(SS2) and (VAR1), there exists some constant $M_2$ such that*

$$N_I^{-1} \sum_{i=1}^{N_I} V_i^2 \quad \leq \quad M_2 N_0^4 n_0^{-2}. \tag{A4}$$

**Lemma 5.** *Under Assumptions (SS0)-(SS2) and (VAR1), there exists some constant $M_3$ such that*

$$N_I^{-1} \sum_{i=1}^{N_I} V(\hat{Y}_i^2) \quad \leq \quad M_3 N_0^4 n_0^{-1}. \tag{A5}$$

**Lemma 6.** *Under Assumptions (SS0)-(SS3) and (VAR1), there exists some constant $M_4$ such that*

$$N_I^{-1} \sum_{i=1}^{N_I} V(\hat{V}_i) \quad \leq \quad M_4 N_0^4 n_0^{-3}. \tag{A6}$$

# 2 Proof of Proposition 6

## 2.1 Some Preliminary Lemmas

We will need the following Lemmas. The proof of Lemma 7 is direct from Assumption (FS1), and is therefore omitted.

**Lemma 7.** *Suppose that Assumption (FS1) holds. Then there exists some constant $c_{I0}$ such that*

$$c_{I0} n_I \quad \leq \quad \sum_{i=1}^{N_I} \pi_{Ii}(1 - \pi_{Ii}) \equiv d_I. \tag{A7}$$

**Lemma 8.** *Suppose that assumptions (FS1), (SS0)-(SS2) and (VAR1) hold. Then*

$$\sum_{i=1}^{N_I} \frac{E(\hat{Y}_i - Y_i)^4}{\pi_{Ii}^3} \quad = \quad O\left(\frac{N^4}{n_I^3}\right). \tag{A8}$$

**Proof .** *We have*

$$E(\hat{Y}_i - Y_i)^4 \quad \leq \quad 16 E(\hat{Y}_i^4) \leq 16 \left\{ V(\hat{Y}_i^2) + 2V_i^2 + 2Y_i^4 \right\}. \tag{A9}$$

*From Assumption (FS1) and from Lemmas 3, 4 and 5, we obtain the result.*

**Lemma 9.** *Suppose that a rejective sampling design is used at the first stage. Suppose that assumptions (FS1), (SS0)-(SS2) and (VAR1) hold. Then we have:*

$$E\left[N^{-2}n_I\left\{\hat{V}_{HAJ,A}(\hat{Y}_\pi)-\tilde{V}_{HAJ,A}(\hat{Y}_\pi)\right\}1(\Omega_r)\right]^2 \;=\; O(n_I^{-1}), \tag{A10}$$

*where*

$$\tilde{V}_{HAJ,A}(\hat{Y}_\pi) \;=\; \sum_{i=1}^{N_I}\pi_{Ii}(1-\pi_{Ii})\left(\frac{\hat{Y}_i}{\pi_{Ii}}-\hat{R}\right)^2, \tag{A11}$$

$$\hat{R} \;=\; d_I^{-1}\sum_{i=1}^{N_I}\pi_{Ii}(1-\pi_{Ii})\frac{\hat{Y}_i}{\pi_{Ii}}, \tag{A12}$$

*and with* $\Omega_r=\{\hat{d}_{rI}\geq\frac{c_{I0}}{2}n_I\}$.

**Proof .** *In this proof, we simplify the notation as* $\hat{V}_{HAJ,A}\equiv\hat{V}_{HA}$ *and* $\tilde{V}_{HAJ,A}\equiv\tilde{V}_{HA}$. *We can write*

$$\left\{\hat{V}_{HA}-\tilde{V}_{HA}\right\}1(\Omega_r) \;=\; T_{A1}-T_{A2}-T_{A3}, \tag{A13}$$

*with*

$$\begin{aligned}
T_{A1} &= \left\{\sum_{i=1}^{N_I}(I_{Ii}-\pi_{Ii})(1-\pi_{Ii})\left(\frac{\hat{Y}_i}{\pi_{Ii}}\right)^2\right\}1(\Omega_r),\\
T_{A2} &= (\hat{d}_{rI}^{-1}-d_I^{-1})\left\{\sum_{i=1}^{N_I}\pi_{Ii}(1-\pi_{Ii})\frac{\hat{Y}_i}{\pi_{Ii}}\right\}^2 1(\Omega_r), \qquad\qquad (A14)\\
T_{A3} &= \hat{d}_{rI}^{-1}\left[\left\{\sum_{i\in S_{rI}}(1-\pi_{Ii})\frac{\hat{Y}_i}{\pi_{Ii}}\right\}^2-\left\{\sum_{i=1}^{N_I}\pi_{Ii}(1-\pi_{Ii})\frac{\hat{Y}_i}{\pi_{Ii}}\right\}^2\right]1(\Omega_r).
\end{aligned}$$

*We consider* $T_{A1}$ *first. We note* $S_{II}=\cup_{i=1}^{N_I}S_i$ *the union of the second-stage samples. We have*

$$\begin{aligned}
E(T_{A1}^2) &\leq E\left[\sum_{i=1}^{N_I}(I_{Ii}-\pi_{Ii})(1-\pi_{Ii})\left(\frac{\hat{Y}_i}{\pi_{Ii}}\right)^2\right]^2\\
&= EV\left[\sum_{i=1}^{N_I}(I_{Ii}-\pi_{Ii})(1-\pi_{Ii})\left(\frac{\hat{Y}_i}{\pi_{Ii}}\right)^2\middle| S_{II}\right]\\
&\leq E\left[\sum_{i=1}^{N_I}\frac{(1-\pi_{Ii})^3}{\pi_{Ii}^3}(\hat{Y}_i)^4\right]\leq\sum_{i=1}^{N_I}\frac{E(\hat{Y}_i)^4}{\pi_{Ii}^3}. \qquad\qquad (A15)
\end{aligned}$$

*From Lemmas 3, 4 and 5, we obtain*

$$E(T_{A1}^2) = O\left(\frac{N^4}{n_I^3}\right). \quad \text{(A16)}$$

*We now consider $T_{A2}$. We obtain*

$$E(T_{A2}^2) \leq \frac{4}{(c_{I0})^4 n_I^4} E(\hat{d}_{rI} - d_I)^2 \times E\left\{\sum_{i=1}^{N_I}(1-\pi_{Ii})\hat{Y}_i\right\}^4. \quad \text{(A17)}$$

*We have*

$$E(\hat{d}_{rI} - d_I)^2 = V(\hat{d}_{rI}) \leq \sum_{i=1}^{N_I} \pi_{Ii} = n_I, \quad \text{(A18)}$$

*and*

$$E\left\{\sum_{i=1}^{N_I}(1-\pi_{Ii})\hat{Y}_i\right\}^4 \leq N_I^3 \sum_{i=1}^{N_I} E(\hat{Y}_i)^4 = O(N^4). \quad \text{(A19)}$$

*From (A17), (A18) and (A19), we obtain*

$$E(T_{A2}^2) = O\left(\frac{N^4}{n_I^3}\right). \quad \text{(A20)}$$

*Finally, we consider $T_{A3}$. We have*

$$E(T_{A3}^2|S_{II}) \leq \frac{4}{(c_{I0})^2 n_I^2}\left(V\left[\left\{\sum_{i\in S_{rI}}(1-\pi_{Ii})\frac{\hat{Y}_i}{\pi_{Ii}}\right\}^2 \middle| S_{II}\right] + \left[V\left\{\sum_{i\in S_{rI}}(1-\pi_{Ii})\frac{\hat{Y}_i}{\pi_{Ii}}\middle| S_{II}\right\}\right]^2\right). \quad \text{(A21)}$$

*By a proof similar to that of Proposition 3, we obtain after some algebra that*

$$E(T_{A3}^2) = O\left(\frac{N^4}{n_I^3}\right). \quad \text{(A22)}$$

*From (A16), (A20) and (A22), we obtain the result.*

**Lemma 10.** *Suppose that a rejective sampling design is used at the first stage. Suppose that assumptions (FS1), (SS0)-(SS2) and (VAR1) hold. Then we have:*

$$E\left[N^{-2} n_I \left\{\tilde{V}_{HAJ,A}(\hat{Y}_\pi)1(\Omega_r) - V_1(\hat{Y}_\pi) - V_2(\hat{Y}_\pi)\right\}\right]^2 = o(1). \quad \text{(A23)}$$

**Proof .** *In this proof, we simplify the notation as* $\tilde{V}_{HAJ,A} \equiv \tilde{V}_{HA}$, $V_1(\hat{Y}_\pi) \equiv V_1$ *and* $V_2(\hat{Y}_\pi) \equiv V_2$. *We can write*

$$\tilde{V}_{HA} 1(\Omega_r) - V_1 - V_2 \;=\; T_{A4} + T_{A5} - T_{A6}, \tag{A24}$$

*with*

$$\begin{aligned} T_{A4} &= \left\{\tilde{V}_{HT,A} - V_1 - V_2\right\} 1(\Omega_r), \\ T_{A5} &= \left\{\tilde{V}_{HA} - \tilde{V}_{HT,A}\right\} 1(\Omega_r), \\ T_{A6} &= \{V_1 + V_2\} 1(\overline{\Omega_r}), \end{aligned} \tag{A25}$$

*where*

$$\tilde{V}_{HT,A} \;\equiv\; \sum_{i,j=1}^{N_I} \frac{\Delta_{Iij}}{\pi_{Ii}\pi_{Ij}} \hat{Y}_i \hat{Y}_j = E\left[\hat{V}_{HT,A}(\hat{Y}_\pi) \middle| S_{II}\right]. \tag{A26}$$

*We consider the term* $T_{A4}$ *first. We have*

$$\begin{aligned} E(T_{A4}^2) &\leq E\left\{\tilde{V}_{HT,A} - V_1 - V_2\right\}^2 = V\left\{\tilde{V}_{HT,A}\right\} \\ &\leq 2V\left[\sum_{i=1}^{N_I} \frac{1-\pi_{Ii}}{\pi_{Ii}} (\hat{Y}_i)^2\right] + 2V\left[\sum_{i\neq j=1}^{N_I} \frac{\Delta_{Iij}}{\pi_{Ii}\pi_{Ij}} \hat{Y}_i \hat{Y}_j\right]. \end{aligned} \tag{A27}$$

*We have*

$$V\left[\sum_{i=1}^{N_I} \frac{1-\pi_{Ii}}{\pi_{Ii}} (\hat{Y}_i)^2\right] \;\leq\; \sum_{i=1}^{N_I} \frac{V\{(\hat{Y}_i)^2\}}{\pi_{Ii}^2}, \tag{A28}$$

*and from Assumption (FS1) and Lemma 5 we obtain*

$$V\left[\sum_{i=1}^{N_I} \frac{1-\pi_{Ii}}{\pi_{Ii}} (\hat{Y}_i)^2\right] \;=\; O\left(\frac{N_I^3 N_0^4}{n_I^2 n_0}\right). \tag{A29}$$

*We also have*

$$\begin{aligned} V\left[\sum_{i\neq j=1}^{N_I} \frac{\Delta_{Iij}}{\pi_{Ii}\pi_{Ij}} \hat{Y}_i \hat{Y}_j\right] &= 2\sum_{i\neq j=1}^{N_I} \sum_{j'\in U_I\setminus\{i,j\}} \frac{\Delta_{Iij}}{\pi_{Ii}\pi_{Ij}} \frac{\Delta_{Iij'}}{\pi_{Ii}\pi_{Ij'}} Cov\left[\hat{Y}_i\hat{Y}_j, \hat{Y}_i\hat{Y}_{j'}\right] \\ &+ \sum_{i\neq j=1}^{N_I} \left(\frac{\Delta_{Iij}}{\pi_{Ii}\pi_{Ij}}\right)^2 V(\hat{Y}_i\hat{Y}_j) \\ &= 2\sum_{i\neq j=1}^{N_I} \sum_{j'\in U_I\setminus\{i,j\}} \frac{\Delta_{Iij}}{\pi_{Ii}\pi_{Ij}} \frac{\Delta_{Iij'}}{\pi_{Ii}\pi_{Ij'}} \left[Y_j Y_{j'} V_i\right] \\ &+ \sum_{i\neq j=1}^{N_I} \left(\frac{\Delta_{Iij}}{\pi_{Ii}\pi_{Ij}}\right)^2 \left[Y_j^2 V_i + Y_i^2 V_j + V_i V_j\right]. \end{aligned} \tag{A30}$$

*From Assumption (FS1), and from Lemmas 4 and 5, we obtain after some algebra*

$$V\left[\sum_{i\neq j=1}^{N_I} \frac{\Delta_{Iij}}{\pi_{Ii}\pi_{Ij}} \hat{Y}_i \hat{Y}_j\right] = O\left(\frac{N_I^3 N_0^4}{n_I^2 n_0}\right). \quad \text{(A31)}$$

*From (A27), (A29) and (A31), we obtain*

$$\begin{aligned} V\left\{\tilde{V}_{HT,A}\right\} &= O\left(\frac{N_I^3 N_0^4}{n_I^2 n_0}\right), \\ E(T_{A4}^2) &= O\left(\frac{N_I^3 N_0^4}{n_I^2 n_0}\right). \quad \text{(A32)} \end{aligned}$$

*We now consider the term $T_{A5}$. From Hájek (1964, Theorem 5.2), we have*

$$\tilde{V}_{HA} = \tilde{V}_{HT,A}\{1+o(1)\}, \quad \text{(A33)}$$

*which leads to*

$$E(T_{A5}^2) \leq E(\tilde{V}_{HT,A})^2 \times o(1). \quad \text{(A34)}$$

*We have*

$$\begin{aligned} E(\tilde{V}_{HT,A})^2 &= V\left\{\tilde{V}_{HT,A}\right\} + [V_1+V_2]^2 \\ &= O\left(\frac{N_I^4 N_0^4}{n_I^2}\right), \quad \text{(A35)} \end{aligned}$$

*where the last line in (A35) follows from equation (A32) and from Proposition 1. This leads to*

$$E(T_{A5}^2) \leq o\left(\frac{N_I^4 N_0^4}{n_I^2}\right). \quad \text{(A36)}$$

*Finally, we consider the term $T_{A6}$. We have*

$$E(T_{A6}^2) \leq (V_1+V_2)^2 Pr(\overline{\Omega_r}). \quad \text{(A37)}$$

*Recall that from Lemma 7, we have $d_I \geq c_{I0} n_I$. Therefore*

$$\begin{aligned} Pr(\overline{\Omega_r}) &= Pr(\hat{d}_{rI} \leq \frac{c_{I0} n_I}{2}) \\ &\leq Pr\left(|\hat{d}_{rI} - d_I| \geq \frac{c_{I0} n_I}{2}\right) \leq \frac{4V(\hat{d}_{rI})}{c_{I0}^2 n_I^2}, \quad \text{(A38)} \end{aligned}$$

*where the last line follows from the Chebyshev inequality. From equations (A18) and (A38), we obtain $Pr(\overline{\Omega_r}) = O(n_I^{-1})$, which along with Proposition 1 leads to*

$$E(T_{A6}^2) = O\left(\frac{N_I^4 N_0^4}{n_I^3}\right). \quad \text{(A39)}$$

*From equations (A32), (A36) and (A39), we obtain the result.*

## 2.2 Proof of Proposition 6

We now consider Proposition 6. We first note that equation (44) follows from Lemmas 9 and 10. Also, equation (46) follows from equations (44) and (28). We therefore focus on proving the asymptotic normality in equation (43). It will follow from Theorem 2.1 in Ohlsson (1989) if we are able to prove his conditions (C1), (C2) and (2.8). With our notation, these conditions are

$$\frac{\tilde{Y}_\pi - Y}{\sqrt{V(\tilde{Y}_\pi)}} \longrightarrow_{\mathcal{L}} \mathcal{N}(0,1), \tag{A40}$$

$$\frac{\sum_{i=1}^{N_I} \frac{E(\hat{Y}_i - Y_i)^4}{\pi_{Ii}^3}}{\left\{V(\hat{Y}_\pi)\right\}^2} \longrightarrow 0, \tag{A41}$$

$$\pi_{Iij} - \pi_{Ii}\pi_{Ij} \leq 0, \tag{A42}$$

where $\tilde{Y}_\pi = \sum_{i \in S_I} \frac{Y_i}{\pi_{Ii}}$. Equation (A42) corresponds to the so-called Yates-Grundy conditions, which is a well-known property of rejective sampling (e.g. Qualité, 2008). Also, equation (A41) follows from equation (A8) in Lemma 8 and from Assumption (VAR2).

It remains to prove equation (A40), namely that the estimator $\tilde{Y}_\pi$ is asymptotically normally distributed. It will follow from the Lyapunov condition

$$\frac{\sum_{i=1}^{N_I} \frac{(Y_i - R\pi_{Ii})^4}{\pi_{Ii}^3}}{\left\{\sum_{i=1}^{N_I} (Y_i - R\pi_{Ii})^2 \left(\frac{1}{\pi_{Ii}} - 1\right)\right\}^2} \longrightarrow 0, \tag{A43}$$

where $R = d_I^{-1} \sum_{i=1}^{N_I} \pi_{Ii}(1-\pi_{Ii}) \frac{Y_i}{\pi_{Ii}}$. From Lemma 3 and assumption (FS1):

$$\sum_{i=1}^{N_I} \frac{(Y_i - R\pi_{Ii})^4}{\pi_{Ii}^3} = O\left(\frac{N^4}{n_I^3}\right). \tag{A44}$$

From Theorem 6.1 in Hájek (1964), we have

$$\sum_{i=1}^{N_I} (Y_i - R\pi_{Ii})^2 \left(\frac{1}{\pi_{Ii}} - 1\right) = V(\tilde{Y}_\pi)\{1 + o(1)\}. \tag{A45}$$

From equations (A44) and (A45) and from assumption (VAR2), we obtain (A43). The proof is complete.

# 3 Proof of Propositions 7, 8 and 9

## 3.1 Some preliminary results

Lemma 11 is stated in van Der Hofstad (2016), for example.

**Lemma 11.** *We have*

$$\begin{aligned}\sum_{s_I \subset U_I} p(s_{pI}) \wedge p_r(s_{pI}) &= 1 - d_{TV}(p, p_r), \\ \sum_{s_I \subset U_I;\; p(s_I) > p_r(s_I)} \{p(s_{pI}) - p_r(s_{pI})\} &= d_{TV}(p, p_r), \\ \sum_{s_I \subset U_I;\; p(s_I) \le p_r(s_I)} \{p_r(s_{pI}) - p(s_{pI})\} &= d_{TV}(p, p_r).\end{aligned} \tag{A46}$$

**Lemma 12.** *Suppose that the first-stage sample is selected by means of rejective sampling. Suppose that assumptions (FS1) and (VAR1) hold. Then*

$$E\left\{\left(\sum_{i \in S_{rI}} \frac{Y_i}{\pi_{Ii}} - Y\right)^4\right\} = O\left(\frac{N^4}{n_I^2}\right). \tag{A47}$$

**Proof .** *We can write*

$$\begin{aligned}E\left(\sum_{i \in S_{rI}} \frac{Y_i}{\pi_{Ii}} - Y\right)^4 &= \sum_{i \in U_I} \left(\frac{Y_i}{\pi_{Ii}}\right)^4 E(I_{Ii} - \pi_{Ii})^4 \\ &+ 4 \sum_{i \neq j = 1}^{N_I} \left(\frac{Y_i}{\pi_{Ii}}\right)^3 \frac{Y_j}{\pi_{Ij}} E\left\{(I_{Ii} - \pi_{Ii})^3 (I_{Ij} - \pi_{Ij})\right\} \\ &+ 3 \sum_{i \neq j = 1}^{N_I} \left(\frac{Y_i}{\pi_{Ii}}\right)^2 \left(\frac{Y_j}{\pi_{Ij}}\right)^2 E\left\{(I_{Ii} - \pi_{Ii})^2 (I_{Ij} - \pi_{Ij})^2\right\} \\ &+ 6 \sum_{i \neq j \neq i' = 1}^{N_I} \left(\frac{Y_i}{\pi_{Ii}}\right)^2 \frac{Y_j}{\pi_{Ij}} \frac{Y_{i'}}{\pi_{Ii'}} E\left\{(I_{Ii} - \pi_{Ii})^2 (I_{Ij} - \pi_{Ij})(I_{Ii'} - \pi_{Ii'})\right\} \\ &+ \sum_{i \neq j \neq i' \neq j' = 1}^{N_I} \frac{Y_i}{\pi_{Ii}} \frac{Y_j}{\pi_{Ij}} \frac{Y_{i'}}{\pi_{Ii'}} \frac{Y_{j'}}{\pi_{Ij'}} E\left\{(I_{Ii} - \pi_{Ii})(I_{Ij} - \pi_{Ij})(I_{Ii'} - \pi_{Ii'})(I_{Ij'} - \pi_{Ij'})\right\}.\end{aligned} \tag{A48}$$

*The result follows from Assumptions (FS1) and (VAR1) and from the following identities:*

$$\begin{aligned}
E(I_{Ii}-\pi_{Ii})^4 &= \pi_{Ii}\{1-\pi_{Ii}\}\{1-3\pi_{Ii}(1-\pi_{Ii})\} \\
&= O\left(\frac{n_I}{N_I}\right), && \text{(A49)} \\
E\left\{(I_{Ii}-\pi_{Ii})^3(I_{Ij}-\pi_{Ij})\right\} &= \{1-3\pi_{Ii}(1-\pi_{Ii})\}\Delta_{Iij} \\
&= O\left(\frac{n_I}{N_I^2}\right), && \text{(A50)} \\
E\left\{(I_{Ii}-\pi_{Ii})^2(I_{Ij}-\pi_{Ij})^2\right\} &= (1-2\pi_{Ii})(1-2\pi_{Ij})\Delta_{Iij} \\
&+ \pi_{Ii}(1-\pi_{Ii})\pi_{Ij}(1-\pi_{Ij}) \\
&= O\left(\frac{n_I^2}{N_I^2}\right), && \text{(A51)} \\
E\left\{(I_{Ii}-\pi_{Ii})^2(I_{Ij}-\pi_{Ij})(I_{Ii'}-\pi_{Ii'})\right\} &= O\left(\frac{n_I^2}{N_I^3}\right), && \text{(A52)} \\
E\left\{(I_{Ii}-\pi_{Ii})(I_{Ij}-\pi_{Ij})(I_{Ii'}-\pi_{Ii'})(I_{Ij'}-\pi_{Ij'})\right\} &= O\left(\frac{n_I^2}{N_I^4}\right), && \text{(A53)}
\end{aligned}$$

*see for example Boistard et al. (2012) for equations (A52) and (A53).*

## 3.2 Proof of Proposition 7

Since $\hat{Y}_{p\pi} = \hat{Y}_{r\pi}$ if $u \leq \alpha$, we have

$$\begin{aligned}
E\left(\hat{Y}_{p\pi}-\hat{Y}_{r\pi}\right)^2 &= (1-\alpha)E\left\{\left(\hat{Y}_{p\pi}-\hat{Y}_{r\pi}\right)^2 \middle| u>\alpha\right\}, \\
&= (1-\alpha)V\left\{\hat{Y}_{p\pi}-\hat{Y}_{r\pi} \middle| u>\alpha\right\}, && \text{(A54)}
\end{aligned}$$

where the second line in (A54) follows from the fact that

$$E\left\{\hat{Y}_{p\pi} \middle| u>\alpha\right\} = E\left\{\hat{Y}_{r\pi} \middle| u>\alpha\right\} \equiv Y_\alpha \text{ (say)}. \quad \text{(A55)}$$

We have

$$\begin{aligned}
V\left\{\hat{Y}_{p\pi}-\hat{Y}_{r\pi} \middle| u>\alpha\right\} &= V\left[E\left\{\hat{Y}_{p\pi}-\hat{Y}_{r\pi} \middle| S_{pI}, S_{rI}, u>\alpha\right\} \middle| u>\alpha\right] \\
&+ E\left[V\left\{\hat{Y}_{p\pi}-\hat{Y}_{r\pi} \middle| S_{pI}, S_{rI}, u>\alpha\right\} \middle| u>\alpha\right] \\
&\equiv V_1+V_2. && \text{(A56)}
\end{aligned}$$

We first consider $V_1$. Since $S_{pI}$ and $S_{rI}$ are independent conditionally on $\{u > \alpha\}$, we obtain

$$\begin{aligned} V_1 &= V\left[\sum_{i\in S_{pI}} \frac{Y_i}{\pi_{Ii}} - \sum_{i\in S_{rI}} \frac{Y_i}{\pi_{Ii}} \middle| u > \alpha\right] \\ &= V\left[\sum_{i\in S_{pI}} \frac{Y_i}{\pi_{Ii}} \middle| u > \alpha\right] + V\left[\sum_{i\in S_{rI}} \frac{Y_i}{\pi_{Ii}} \middle| u > \alpha\right]. \end{aligned} \tag{A57}$$

For the first term in the right-hand side of (A57), we have

$$\begin{aligned} V\left[\sum_{i\in S_{pI}} \frac{Y_i}{\pi_{Ii}} \middle| u > \alpha\right] &= \sum_{\substack{s_I\subset U_I \\ p(s_I)>p_r(s_I)}} \frac{p(s_I)-p_r(s_I)}{1-\alpha} \left(\sum_{i\in s_I} \frac{Y_i}{\pi_{Ii}} - Y_\alpha\right)^2 \\ &\leq \sum_{\substack{s_I\subset U_I \\ p(s_I)>p_r(s_I)}} \frac{p(s_I)-p_r(s_I)}{1-\alpha} \left(\sum_{i\in s_I} \frac{Y_i}{\pi_{Ii}} - Y\right)^2. \end{aligned} \tag{A58}$$

Similarly, we have

$$V\left[\sum_{i\in S_{rI}} \frac{Y_i}{\pi_{Ii}} \middle| u > \alpha\right] \leq \sum_{\substack{s_I\subset U_I \\ p(s_I)\leq p_r(s_I)}} \frac{p_r(s_I)-p(s_I)}{1-\alpha} \left(\sum_{i\in s_I} \frac{Y_i}{\pi_{Ii}} - Y\right)^2,$$

and from (A57) this leads to

$$V_1 \leq \frac{1}{1-\alpha} \sum_{s_I\subset U_I} |p(s_I)-p_r(s_I)| \left(\sum_{i\in s_I} \frac{Y_i}{\pi_{Ii}} - Y\right)^2. \tag{A59}$$

Now, we consider $V_2$. Since the second-stage samples are independent conditionally on $\{u > \alpha\}, S_{pI}$ and $S_{rI}$, we obtain

$$\begin{aligned} V_2 &= E\left[\sum_{i\in S_{pI}} \frac{V_i}{\pi_{Ii}^2} \middle| u > \alpha\right] + E\left[\sum_{i\in S_{rI}} \frac{V_i}{\pi_{Ii}^2} \middle| u > \alpha\right] \\ &= \sum_{\substack{s_I\subset U_I \\ p(s_I)>p_r(s_I)}} \frac{p(s_I)-p_r(s_I)}{1-\alpha} \sum_{i\in s_I} \frac{V_i}{\pi_{Ii}^2} + \sum_{\substack{s_I\subset U_I \\ p(s_I)\leq p_r(s_I)}} \frac{p_r(s_I)-p(s_I)}{1-\alpha} \sum_{i\in s_I} \frac{V_i}{\pi_{Ii}^2}, \end{aligned}$$

which leads to

$$V_2 = \frac{1}{1-\alpha} \sum_{s_I\subset U_I} |p(s_I)-p_r(s_I)| \sum_{i\in s_I} \frac{V_i}{\pi_{Ii}^2}. \tag{A60}$$

From (A54), (A56), (A59) and (A60), the proof is complete.

## 3.3 Proof of Proposition 8

From Proposition 7 and by using the Cauchy-Schwarz inequality, we obtain

$$\begin{aligned}
E\left(\hat{Y}_{p\pi}-\hat{Y}_{r\pi}\right)^2 &\leq \sum_{\substack{s_I\subset U_I\\ p_r(s_I)>0}} \frac{|p(s_I)-p_r(s_I)|}{\sqrt{p_r(s_I)}}\sqrt{p_r(s_I)}\left\{\left(\sum_{i\in s_I}\frac{Y_i}{\pi_{Ii}}-Y\right)^2+\sum_{i\in s_I}\frac{V_i}{\pi_{Ii}^2}\right\} \\
&\leq \sqrt{d_2(p,p_r)}\times\sqrt{2\sum_{s_I\subset U_I}p_r(s_I)\left\{\left(\sum_{i\in s_I}\frac{Y_i}{\pi_{Ii}}-Y\right)^4+\left(\sum_{i\in s_I}\frac{V_i}{\pi_{Ii}^2}\right)^2\right\}}, \\
&= \sqrt{2d_2(p,p_r)}\times\sqrt{E\left(\sum_{i\in S_{rI}}\frac{Y_i}{\pi_{Ii}}-Y\right)^4+E\left(\sum_{i\in S_{rI}}\frac{V_i}{\pi_{Ii}^2}\right)^2}.
\end{aligned}$$

We have

$$E\left(\sum_{i\in S_{rI}}\frac{V_i}{\pi_{Ii}^2}\right)^2 \leq n_I\sum_{i=1}^{N_I}\frac{V_i^2}{\pi_{Ii}^3}=O\left(\frac{N^4}{n_I^2 n_0^2}\right) \tag{A61}$$

where the order of magnitude follows from assumption (FS1) and from Lemma 4. From Lemma 12 and since $d_2(p,p_r)=o(1)$, we obtain (51). Equation (52) follows from equation (51), from Assumption (VAR2) and from the identity

$$\left(\sqrt{V(\hat{Y}_{p\pi})}-\sqrt{V(\hat{Y}_{r\pi})}\right)^2 \leq E\left(\hat{Y}_{p\pi}-\hat{Y}_{r\pi}\right)^2. \tag{A62}$$

## 3.4 Proof of Proposition 9

Equation (53) follows directly from equation (43) in Proposition 6 and from Proposition 8. For equation (54), and by using equation (46), it is sufficient to prove that

$$E\left|\hat{V}_{HAJ}(\hat{Y}_{p\pi})-\hat{V}_{HAJ}(\hat{Y}_{r\pi})\right| = o\left(\frac{N^2}{n_I}\right), \tag{A63}$$

where the samples $S_{rI}$ and $S_{pI}$ are selected by means of the coupling procedure in Algorithm 1. We have

$$\left|\hat{V}_{HAJ}(\hat{Y}_{p\pi})-\hat{V}_{HAJ}(\hat{Y}_{r\pi})\right| = 1(S_{pI}\neq S_{rI})\left|\hat{V}_{HAJ}(\hat{Y}_{p\pi})-\hat{V}_{HAJ}(\hat{Y}_{r\pi})\right|,$$

which from the Cauchy-Schwartz inequality leads to

$$E\left|\hat{V}_{HAJ}(\hat{Y}_{p\pi})-\hat{V}_{HAJ}(\hat{Y}_{r\pi})\right| \leq \sqrt{Pr(S_{pI}\neq S_{rI})}\sqrt{2E\{\hat{V}_{HAJ}(\hat{Y}_{p\pi})\}^2+2E\{\hat{V}_{HAJ}(\hat{Y}_{r\pi})\}^2}.$$

After some straightforward algebra, we obtain

$$E\left|\hat{V}_{HAJ}(\hat{Y}_{p\pi}) - \hat{V}_{HAJ}(\hat{Y}_{r\pi})\right| \leq 2\sqrt{Pr(S_{pI} \neq S_{rI})}\sqrt{n_I \sum_{i=1}^{N_I} \frac{V(\hat{Y}_i^2) + 2V_i^2 + 2Y_i^4}{\pi_{Ii}^3}}.$$

From Lemmas 3 to 5, we have

$$n_I \sum_{i=1}^{N_I} \frac{V(\hat{Y}_i^2) + 2V_i^2 + 2Y_i^4}{\pi_{Ii}^3} \quad = \quad O\left(\frac{N^4}{n_I^2}\right). \tag{A64}$$

Also,

$$Pr(S_{pI} \neq S_{rI}) \quad \leq \quad d_{TV}(p, p_r) \leq \sqrt{d_2(p, p_r)} = o(1), \tag{A65}$$

which completes the proof.

# References


Boistard, H., Lopuhaä, H. P., and Ruiz-Gazen, A. (2012). Approximation of rejective sampling inclusion probabilities and application to high order correlations. *Electron. J. Statist.*, 6:1967–1983.

Hájek, J. (1964). Asymptotic theory of rejective sampling with varying probabilities from a finite population. *Annals of Mathematical Statistics*, 35:1491–1523.

Ohlsson, E. (1989). Asymptotic normality for two-stage sampling from a finite population. *Probability Theory and Related Fields*, 81(3):341–352.

Qualité, L. (2008). A comparison of conditional poisson sampling versus unequal probability sampling with replacement. *Journal of Statistical Planning and Inference*, 138(5):1428 – 1432.

van Der Hofstad, R. (2016). *Random graphs and complex networks.* Cambridge series in statistical and probabilistic mathematics.
